# Supplementary material for: Digging into Depth Priors for Outdoor Neural Radiance Fields
Source: arXiv:2308.04413 source file (2023-08-08)
Supplement: Supplementary file 1 [file 6_Supplementary.tex]

\section{Implementation Details} % moved to supplementary
\noindent \textbf{NeRF Method} For both KITTI~\cite{geiger2012KITTI} and Argoverse~\cite{wilson2023argoverse} dataset, we train the mentioned methods on the selected sequences with a fixed number of steps and evaluate the testing viewpoints in terms of photorealistic metrics and depth accuracy metrics. Specifically, we train MipNeRF-360 for 75,000 iterations with a depth weight of 10 using the official codebase\footnote{\url{https://github.com/google-research/multinerf}}. 
For Instant-NGP, we use the PyTorch re-implemented version\footnote{\url{https://github.com/kwea123/ngp\_pl}}. The model is trained for 30 epochs with a depth weight of 0.5. %, which is trained with a single NVIDIA RTX 3090 GPU.
All of the experiments are performed with Tesla V100 GPUs.

\noindent \textbf{Depth Method} For both KITTI~\cite{geiger2012KITTI} and Argoverse~\cite{wilson2023argoverse} dataset, we firstly re-split the training and testing dataset according to the selected sequence, i.e., using the selected sequence as the testing dataset and the rest as the training dataset. Then, we retrain the mentioned methods with their official implementation of BTS\footnote{\url{https://github.com/cleinc/bts}}, CFNet\footnote{\url{ https://github.com/gallenszl/CFNet}}, PCWNet\footnote{\url{https://github.com/gallenszl/PCWNet}}, and re-implement MFFNet by ourselves. Note that for all generated depth maps, we crop the sky area which has an infinite distance and has no ground supervision. For binocular depth estimation, we select CFNet and PCWNet as the representative work in KITTI and Argoverse datasets, respectively. All of the experiments are performed with Tesla V100 GPUs.

\section{Detailed Experinmental Result}
In this section, we will specifically introduce the used sequence in the two publicly available datasets and the corresponding result.
\subsection{Dataset}
\topic{KITTI:} For the KITTI dataset, We use the following sequences:
\begin{enumerate}
    \item Seq00\_2011\_10\_03\_drive\_0027\_sync: frame 657 - 787 
    \item Seq00\_2011\_10\_03\_drive\_0027\_sync: frame 890 - 1028
    \item Seq00\_2011\_10\_03\_drive\_0027\_sync: frame 2700 - 3000
    \item Seq02\_2011\_10\_03\_drive\_0034\_sync: frame 2749 - 2929
    \item Seq05\_2011\_09\_30\_drive\_0018\_sync: frame 400 - 725
\end{enumerate}

\topic{Argoverse} For the Argoverse dataset, We use all frames in the following sequence:
\begin{enumerate}
    \item Training set: 2c07fcda-6671-3ac0-ac23-4a232e0e031e
    \item Validation set: 70d2aea5-dbeb-333d-b21e-76a7f2f1ba1c
    \item Validation set: cb0cba51-dfaf-34e9-a0c2-d931404c3dd8
\end{enumerate}

\subsection{Additional Results}
The corresponding results in each sequence are shown in Tab. \ref{tab:kittisupp} and Tab.\ref{tab:argosupp}. The conclusions in each sequence are consistent with the results reported in Tab.3 and Tab.5 of the main paper. Consequently, these results further support our finding1: Monocular depth is enough for sparse viewpoints (lines 735-743 of the main paper) and finding2: depth supervision is an option for dense viewpoints (lines 779-786 of the main paper). 

% To further verify our findings, We also experimented with another representative method: NeRF++~\cite{zhang2020nerf++} on the Kitti dataset. Specifically, NeRF++\cite{zhang2020nerf++} divides the unbounded scenes into two volumes: an inner unit sphere and an outer volume. Therefore, the volume rendering also consists of two parts. We render the depth in NeRF++ with an extended version of \equref{equ:depth_render}:
% \begin{gather}
% \begin{aligned}
%     &\mathbf{D}(\mathbf{r}) = \int_{t = 0}^{t^{\prime}} \sigma(\mathbf{r}(t))t \cdot e^{-\int_{s=0}^{s}\sigma(\mathbf{r}(s))\mathrm{d}s} \mathrm{d}t \quad + \\
%     &e^{-\int_{s=0}^{t^{\prime}}\sigma(\mathbf{r}(s))\mathrm{d}s} \cdot \int_{t = t^{\prime}}^{\infty} \sigma(\mathbf{r}(t))t \cdot e^{-\int_{s=t^{\prime}}^{s}\sigma(\mathbf{r}(s))\mathrm{d}s} \mathrm{d}t,
% \end{aligned}
% \label{equ:depth_render}
% \end{gather}
% where $t \in (0, t^{\prime})$ is inside the sphere and $t \in (t^{\prime}, \infty)$ is the unbounded area. The corresponding results are shown in Tab.\ref{tab:nerfppkitti}, which is in compliance with our finding1 and finding2.

\begin{figure*}
    \centering
    \includegraphics[width=0.95\textwidth]{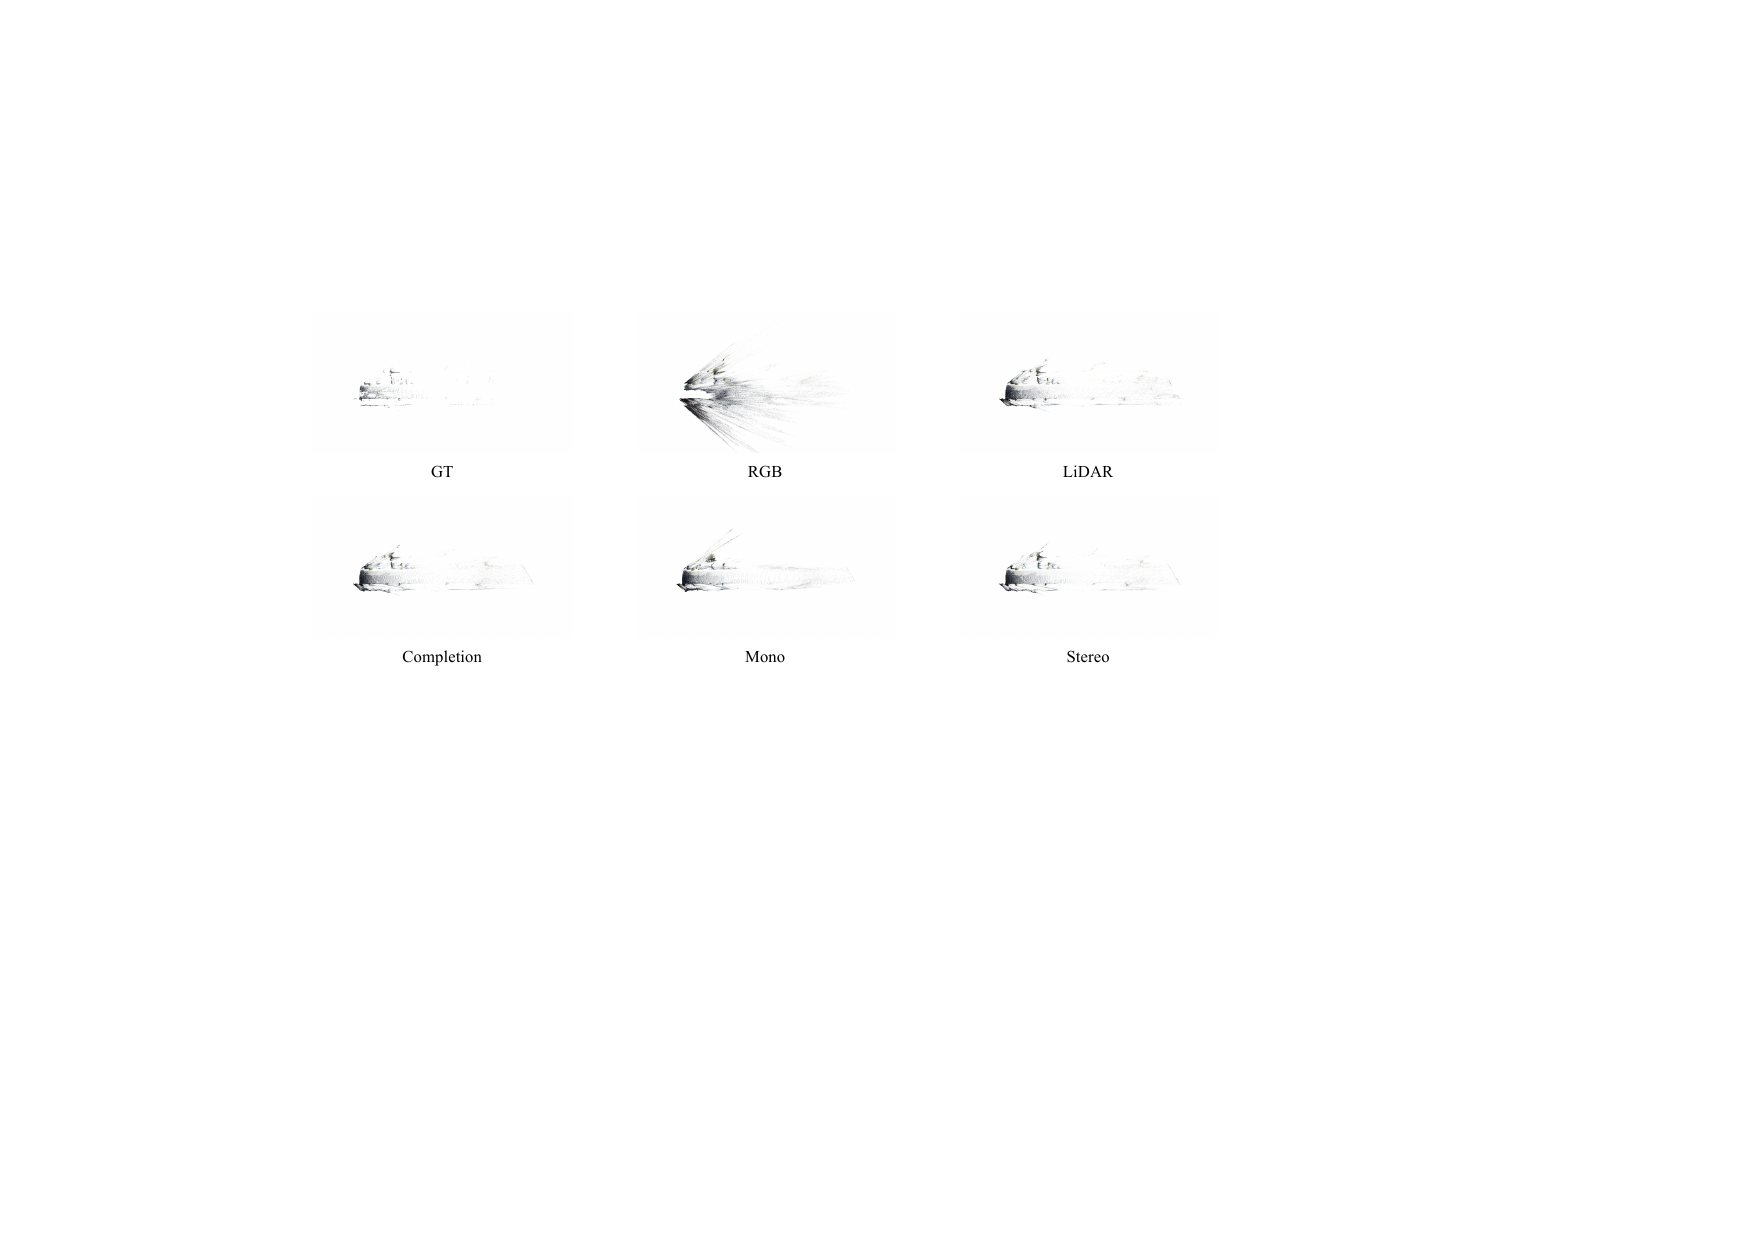}
    \caption{Point cloud visualization of MipNeRF-360 under different depth supervision.}
    \label{fig:pc}
    % \vspace{-0.1in}
\end{figure*}

\section{Detailed Ablation study}
In our \emph{finding 4} of the main paper(lines 904-909), we claim that directly cropping the sky area with MSE supervision is enough. To further validate our claim, we investigate the influence of the cropping-based depth filtering strategy on all depth priors. The corresponding results are shown in Tab. \ref{tab:crop}. Note that because the raw LiDAR supervision originally does not have a valid value in the sky area, we exclude the corresponding results. It can be seen from the table that the cropping-based depth filtering strategy is beneficial for the performance of all depth priors, which verifies our finding. Moreover, as the estimation result of sky area is worse in monocular depth estimation and depth completion, the depth filtering strategy achieves a larger gain in these two depth priors.

\section{More visualization}
We visualize the point clouds for different depth supervision, which can be seen in Fig.~\ref{fig:pc}. We can see that when using only RGB, the point clouds are extremely scattered and shows inaccurate geometry. Adding additional depth supervision will greatly alleviate this problem and helps NeRFs converge to a better geometry.

We also give a more qualitative comparison between different depth priors, which can be seen in Tab. 4 of the main paper. As shown in Fig. \ref{fig:KITTI_res}, depth completion achieves the best accuracy in GT valid area and then goes with binocular depth estimation and monocular depth estimation, which is consistent with the qualitative results. However, depth completion and monocular depth estimation cannot generate reasonable results in gt invalid area, i.e., the sky area. Hence, we need the cropping-based depth filtering strategy to filter out the unreasonable area. Tab. \ref{tab:crop} shows the effectiveness of the proposed method.

% \section{Complete Results}
\begin{table}
\caption{Detailed ablation study of the proposed cropping-based depth filtering strategy on all depth priors.}
\centering
\resizebox{\linewidth}{!}{%
\begin{tabular}{lccccc}
\toprule
& PSNR$\uparrow$ & SSIM$\uparrow$ & LPIPS$\downarrow$ & RMSE$\downarrow$ & Absrel$\downarrow$ \\
RGB & 14.80 & 0.475 & 0.551 & 4.569 & 0.153 \\ \midrule
Completion& 17.98 & 0.540 & 0.540 & 1.057 & \textbf{0.038} \\
Completion Crop & \textbf{18.39} & \textbf{0.554} & \textbf{0.505} & \textbf{1.051} & \textbf{0.038} \\ \midrule
Mono & 17.12 & 0.510 & 0.543 & 2.492 & 0.075 \\
Mono Crop & \textbf{17.97} & \textbf{0.542} & \textbf{0.510} & \textbf{2.383} & \textbf{0.073} \\ \midrule
Stereo & 18.80 & \textbf{0.562} & 0.508 & \textbf{1.347} & 0.042 \\
Stereo Crop & \textbf{18.87} & \textbf{0.562} & \textbf{0.501} & 1.349 & \textbf{0.040} \\
\bottomrule
\end{tabular}
} 
\label{tab:crop}
\end{table}

\begin{table*}
\caption{Quantitative comparison with selected methods on each sequence of KITTI dataset. The best results are bolded.}
\centering
\resizebox{\textwidth}{!}{%
\begin{tabular}{lllccccccccccccccc}
\toprule
& & & \multicolumn{5}{c}{Dense} & \multicolumn{5}{c}{Sparse} \\ Method & Sequence& Depth Supervision & PSNR$\uparrow$ & SSIM$\uparrow$ & LPIPS$\downarrow$ & RMSE$\downarrow$ & Absrel$\downarrow$ & PSNR$\uparrow$ & SSIM$\uparrow$ & LPIPS$\downarrow$ & RMSE$\downarrow$ & Absrel$\downarrow$ \\
\cmidrule(lr){1-1}
\cmidrule(lr){2-2}
\cmidrule(lr){3-3}
\cmidrule(lr){4-8}
% \cmidrule(lr){8-12}
\cmidrule(lr){9-13}
\multirow{25}{*}{MipNeRF-360~\cite{barron2022mip}} & \multirow{5}{*}{(1)} & RGB-Only  & \textbf{22.66} & \textbf{0.755} & \textbf{0.403} & 3.719 & 0.112 & 16.54 & 0.640 & 0.480 & 6.284 & 0.174 \\
&& GT Depth & 22.30 & 0.744 & 0.420 & 0.644 & 0.022& 20.08 & \textbf{0.696} & \textbf{0.446} & 0.714 & 0.026 \\
&& Depth Completion & 21.71 & 0.723 & 0.453 & \textbf{0.627} & \textbf{0.018} & \textbf{20.38} & 0.694 & 0.467 & \textbf{0.651} & \textbf{0.020} \\
&& Stereo Depth & 21.71 & 0.720 & 0.457 & 1.219 & 0.026& 20.40 & 0.691 & 0.469 & 1.264 & 0.028 \\
&& Mono Depth  & 21.73 & 0.723 & 0.449 & 2.362 & 0.056& 19.79 & 0.681 & 0.468 & 2.418 & 0.061 \\
\cmidrule{2-13}
 & \multirow{5}{*}{(2)} & RGB-Only          & \textbf{21.57} & \textbf{0.683} & \textbf{0.406} & 2.656 & 0.058 & 16.86 & 0.579 & 0.467 & 3.704 & 0.106\\
 &  & GT Depth        & 21.48 & 0.673 & 0.421 & 0.821 & 0.020  & \textbf{19.18} & \textbf{0.621} & \textbf{0.441} & 0.876 & 0.025 \\
  &  & Depth Completion  & 21.01 & 0.650 & 0.452 & \textbf{0.711} & \textbf{0.017} & 19.16 & 0.612 & 0.465 & \textbf{0.811} & \textbf{0.019} \\
   &  & Stereo Depth      & 20.93 & 0.648 & 0.455 & 1.224 & 0.022& 19.17 & 0.612 & 0.466 & 1.256 & 0.025 \\
 &  & Mono Depth        & 21.14 & 0.651 & 0.451 & 2.096 & 0.053& 18.60 & 0.600 & 0.470 & 2.197 & 0.057 \\
 \cmidrule{2-13}
 & \multirow{5}{*}{(3)} & RGB-Only & \textbf{21.83} & \textbf{0.641} & \textbf{0.460} & 2.482 & 0.071& 14.80 & 0.475 & 0.551 & 4.569 & 0.153 \\
 &  & GT Depth & 21.56 & 0.629 & 0.473 & 1.015 & 0.036 & 17.47 & 0.542 & 0.507 & 1.173 & 0.045  \\
  &  & Depth Completion  & 21.26 & 0.621 & 0.482 & \textbf{0.894} & \textbf{0.030} & 18.39 & 0.554 & 0.505 & \textbf{1.051} & \textbf{0.038} \\
  &  & Stereo Depth      & 21.40 & 0.621 & 0.482 & 1.249 & 0.033 & \textbf{18.87} & \textbf{0.562} & \textbf{0.501} & 1.349 & 0.040 \\
 &  & Mono Depth        & 21.15 & 0.615 & 0.486 & 2.287 & 0.062 & 17.97 & 0.542 & 0.510 & 2.383 & 0.073 \\
 \cmidrule{2-13}
 & \multirow{5}{*}{(4)} & RGB-Only          & 21.61 & \textbf{0.678} & \textbf{0.466} & 4.050 & 0.115 & 17.81 & 0.609 & 0.502 & 5.386 & 0.170 \\
 &  & GT Depth         & \textbf{21.67} & 0.672 & 0.474 & 1.009 & 0.040  & 19.29 & 0.631 & 0.491 & 1.267 & 0.055 \\
&  & Depth Completion & 21.60 & 0.669 & 0.479 & \textbf{0.946} & \textbf{0.031} & \textbf{19.74} & \textbf{0.636} & \textbf{0.489} & \textbf{1.049} & \textbf{0.036} \\
&  & Stereo Depth      & 21.59 & 0.669 & 0.480 & 1.181 & 0.035 & 19.69 & \textbf{0.636} & 0.491 & 1.315 & 0.038\\
 &  & Mono Depth       & 21.59 & 0.667 & 0.481 & 1.953 & 0.057& 19.61 & 0.632 & 0.492 & 2.026 & 0.063 \\
 \cmidrule{2-13}
 & \multirow{5}{*}{(5)} & RGB-Only         & \textbf{22.30} & \textbf{0.702} & \textbf{0.453} & 2.543 & 0.084 & 18.65 & 0.643 & 0.491 & 3.370 & 0.116 \\
 &  & GT Depth          & 22.19 & 0.693 & 0.465 & 1.099 & 0.043& 19.71 & 0.657 & 0.485 & 1.193 & 0.050 \\
  &  & Depth Completion  & 21.99 & 0.689 & 0.470 & \textbf{0.912} & \textbf{0.033} & 20.57 & 0.663 & 0.484 & \textbf{0.975} & \textbf{0.037} \\
 &  & Stereo Depth      & 22.03 & 0.688 & 0.470 & 1.090 & \textbf{0.033} & \textbf{20.62} & \textbf{0.665} & \textbf{0.481} & 1.148 & 0.038 \\
 &  & Mono Depth        & 21.81 & 0.685 & 0.473 & 2.106 & 0.068& 20.20 & 0.655 & 0.488 & 2.194 & 0.076 \\
\midrule
\multirow{25}{*}{InstantNGP~\cite{muller2022instant}} & \multirow{5}{*}{(1)} 
& RGB-Only  & 21.59 & 0.701 & 0.433 & 9.352 & 0.534 & 14.74 & 0.543 & 0.534 & 14.020 & 0.727 \\
&& GT Depth & \textbf{21.84} & \textbf{0.705} & \textbf{0.429} & \textbf{0.985} & \textbf{0.032} & \textbf{19.35} & \textbf{0.652} & \textbf{0.454} & \textbf{1.083} & 0.036 \\ 
&& Depth Completion & 21.31 & 0.684 & 0.462 & 1.041 & \textbf{0.032} & 19.33 & 0.638 & 0.487 & 1.106 & \textbf{0.035} \\
&& Stereo Depth & 21.19 & 0.677 & 0.467 & 1.311 & 0.044 & 19.13 & 0.629 & 0.492 & 1.384 & 0.046 \\
&& Mono Depth & 20.59 & 0.658 & 0.478 & 2.457 & 0.062 & 18.62 & 0.606 & 0.500 & 2.571 & 0.067 \\

\cmidrule{2-13}
 & \multirow{5}{*}{(2)} & RGB-Only & 20.45 & 0.621 & 0.426 & 9.141 & 0.479 & 13.28 & 0.418 & 0.555 & 15.783 & 0.832 \\
&& GT Depth & \textbf{21.02} & \textbf{0.641} & \textbf{0.408} & \textbf{0.913} & 0.026 & 18.06 & \textbf{0.570} & \textbf{0.436} & \textbf{1.117} & 0.035  \\
&& Depth Completion & 20.77 & 0.624 & 0.441 & 0.986 & \textbf{0.024} & \textbf{18.23} & 0.560 & 0.464 & 1.204 & \textbf{0.032}  \\
&& Stereo Depth & 20.94 & 0.620 & 0.440 & 1.253 & 0.032 & 18.11 & 0.558 & 0.467 & 1.471 & 0.040  \\
&& Mono Depth & 20.53 & 0.607 & 0.456 & 2.108 & 0.064 & 17.77 & 0.535 & 0.480 & 2.371 & 0.077  \\
 \cmidrule{2-13}
 & \multirow{5}{*}{(3)} 
 & RGB-Only & 20.70 & 0.644 & 0.471 & 9.338 & 0.475 & 16.47 & 0.554 & 0.510 & 14.919 & 0.810  \\
&& GT Depth & \textbf{21.53} & \textbf{0.658} & \textbf{0.457} & \textbf{1.365} & 0.055 & 18.63 & 0.596 & \textbf{0.481} & 1.715 & 0.070  \\
&& Depth Completion & 21.47 & 0.652 & 0.468 & 1.398 & \textbf{0.047} & \textbf{19.06} & \textbf{0.603} & 0.483 & \textbf{1.593} & \textbf{0.056}  \\
&& Stereo Depth & 21.36 & 0.649 & 0.472 & 1.398 & 0.050 & \textbf{19.06} & 0.599 & 0.484 & 1.698 & 0.062  \\
&& Mono Depth & 21.42 & 0.647 & 0.475 & 2.175 & 0.072 & 18.85 & 0.593 & 0.489 & 2.451 & 0.085  \\
 \cmidrule{2-13}
 & \multirow{5}{*}{(4)} & RGB-Only & 17.65 & 0.502 & 0.526 & 10.861 & 0.494 & 13.47 & 0.360 & 0.600 & 16.730 & 0.806  \\
&& GT Depth & \textbf{19.65} & \textbf{0.548} & \textbf{0.496} & \textbf{3.475} & \textbf{0.101} & \textbf{16.63} & \textbf{0.464} & \textbf{0.518} & \textbf{3.589} & \textbf{0.108}  \\
&& Depth Completion & 19.14 & 0.531 & 0.515 & 3.613 & 0.102 & 16.59 & 0.454 & 0.537 & 3.866 & 0.116  \\
&& Stereo Depth & 19.39 & 0.530 & 0.514 & 3.760 & 0.111 & 16.87 & 0.455 & 0.536 & 3.774 & 0.117  \\
&& Mono Depth & 18.95 & 0.517 & 0.525 & 4.262 & 0.135 & 16.40 & 0.442 & 0.540 & 4.405 & 0.147  \\
 \cmidrule{2-13}
 & \multirow{5}{*}{(5)} & RGB-Only & 22.17 & 0.681 & 0.445 & 9.180 & 0.555 & 19.23 & 0.620 & 0.481 & 13.604 & 0.792  \\
&& GT Depth & \textbf{22.47} & \textbf{0.697} & \textbf{0.431} & \textbf{1.115} & 0.047 & \textbf{19.96} & \textbf{0.646} & \textbf{0.458} & \textbf{1.250} & \textbf{0.053}  \\
&& Depth Completion & 21.78 & 0.671 & 0.464 & 1.268 & \textbf{0.045} & 19.88 & 0.625 & 0.487 & 1.393 & 0.055  \\
&& Stereo Depth & 21.80 & 0.671 & 0.465 & 1.429 & 0.048 & 19.81 & 0.626 & 0.488 & 1.596 & 0.056  \\
&& Mono Depth & 21.46 & 0.657 & 0.479 & 2.395 & 0.095 & 19.21 & 0.610 & 0.499 & 2.540 & 0.104  \\
\bottomrule
\end{tabular}
} 
\label{tab:kittisupp}
\end{table*}

\begin{table*}
\caption{Quantitative comparison with selected methods on each sequence of Argoverse dataset. The best results are bolded.}
\centering
\resizebox{\textwidth}{!}{%
\begin{tabular}{lllccccccccccccccc}
\toprule
& & & \multicolumn{5}{c}{Dense} & \multicolumn{5}{c}{Sparse} \\ Method & Sequence& Depth Supervision & PSNR$\uparrow$ & SSIM$\uparrow$ & LPIPS$\downarrow$ & RMSE$\downarrow$ & Absrel$\downarrow$ & PSNR$\uparrow$ & SSIM$\uparrow$ & LPIPS$\downarrow$ & RMSE$\downarrow$ & Absrel$\downarrow$ \\
\cmidrule(lr){1-1}
\cmidrule(lr){2-2}
\cmidrule(lr){3-3}
\cmidrule(lr){4-8}
% \cmidrule(lr){8-12}
\cmidrule(lr){9-13}
\multirow{12}{*}{MipNeRF-360~\cite{barron2022mip}} & \multirow{4}{*}{(1)} & RGB-Only     & \textbf{27.81} & \textbf{0.839} & \textbf{0.459} & 5.253 & 0.114 & 24.60 & 0.819 & 0.480 & 6.158 & 0.136\\
 &  & GT Depth      & 27.39 & 0.830 & 0.469 & \textbf{1.735} & \textbf{0.041} & \textbf{26.35} & \textbf{0.824} & \textbf{0.474} & \textbf{1.812} & \textbf{0.043} \\
  &  & Stereo Depth  & 26.81 & 0.820 & 0.482 & 3.173 & 0.056 & 26.31 & 0.817 & 0.483 & 3.194 & 0.058 \\
 &  & Mono Depth    & 27.15 & 0.825 & 0.481 & 3.866 & 0.078 & 26.59 & 0.821 & 0.481 & 4.085 & 0.077 \\
 \cmidrule{2-13}
 & \multirow{4}{*}{(2)} & RGB-Only      & \textbf{29.42} & \textbf{0.865} & \textbf{0.430} & 6.884 & 0.129 & 24.44 & 0.822 & 0.458 & 8.185 & 0.144\\
 &  & GT Depth      & 28.91 & 0.856 & 0.443 & \textbf{3.073} & \textbf{0.056} & \textbf{28.03} & \textbf{0.849} & \textbf{0.446} & \textbf{3.571} & \textbf{0.062} \\
&  & Stereo Depth  & 28.52 & 0.849 & 0.452 & 4.670 & 0.061 & 27.46 & 0.841 & 0.452 & 4.841 & 0.068 \\
 &  & Mono Depth    & 28.76 & 0.852 & 0.446 & 5.004 & 0.096 & 27.94 & 0.844 & 0.450 & 5.338 & 0.096 \\
 \cmidrule{2-13}
 & \multirow{4}{*}{(3)} & RGB-Only      & \textbf{30.81} & \textbf{0.863} & \textbf{0.448} & 6.204 & 0.118 & 28.40 & 0.845 & \textbf{0.466} & 6.569 & 0.137 \\
 &  & GT Depth     & 30.04 & 0.852 & 0.464 & \textbf{1.944} & \textbf{0.037}  & \textbf{29.64} & \textbf{0.848} & 0.467 & \textbf{1.947} & \textbf{0.039} \\
  &  & Stereo Depth  & 29.63 & 0.843 & 0.476 & 4.970 & 0.076 & 29.40 & 0.841 & 0.477 & 4.895 & 0.074 \\
 &  & Mono Depth    & 29.84 & 0.846 & 0.472 & 4.957 & 0.106 & 29.59 & 0.844 & 0.472 & 5.181 & 0.106\\
\midrule
\multirow{12}{*}{InstantNGP~\cite{muller2022instant}} & \multirow{4}{*}{(1)} 
& RGB-Only & 25.85 & \textbf{0.823} & 0.482 & 18.462 & 0.774 & 22.03 & 0.804 & 0.505 & 19.026 & 0.751 \\
&& GT Depth  & \textbf{27.83} & \textbf{0.823} & \textbf{0.473} & \textbf{1.947} & \textbf{0.061} & \textbf{26.30} & 0.811 & 0.482 & \textbf{2.018} & \textbf{0.066} \\
&& Stereo Depth  & 27.21 & 0.817 & 0.478 & 5.365 & 0.091& 26.04 & \textbf{0.814} & \textbf{0.481} & 5.535 & 0.100 \\
&& Mono Depth  & 27.03 & 0.816 & 0.486 & 5.653 & 0.113 & 25.71 & 0.808 & 0.488 & 5.812 & 0.112\\

 \cmidrule{2-13}
 & \multirow{4}{*}{(2)} 
& RGB-Only  & 28.40 & \textbf{0.867} & \textbf{0.424} & 8.804 & 0.263 & 24.38 & 0.844 & 0.449 & 11.884 & 0.378\\
&& GT Depth  & \textbf{28.56} & \textbf{0.867} & 0.426 & \textbf{1.993} & \textbf{0.043} & \textbf{26.97} & \textbf{0.849} & \textbf{0.440} & \textbf{1.934} & \textbf{0.043} \\
&& Stereo Depth  & 27.83 & 0.857 & 0.441 & 4.977 & 0.075& 26.28 & 0.839 & 0.452 & 5.386 & 0.082 \\
&& Mono Depth  & 28.27 & 0.859 & 0.442 & 5.612 & 0.111 & 26.48 & 0.845 & 0.451 & 6.469 & 0.129\\
 
 \cmidrule{2-13}
 & \multirow{4}{*}{(3)}
& RGB-Only  & 29.96 & \textbf{0.851} & \textbf{0.445} & 13.167 & 0.443 & 20.12 & 0.800 & 0.528 & 21.407 & 0.650 \\
&& GT Depth  & \textbf{30.38} & 0.850 & 0.449 & \textbf{1.471} & \textbf{0.031} & 28.88 & \textbf{0.842} & \textbf{0.457} & \textbf{1.691} & \textbf{0.035} \\
&& Stereo Depth  & 29.93 & 0.843 & 0.460 & 6.497 & 0.104& \textbf{28.98} & 0.831 & 0.470 & 6.610 & 0.109 \\
&& Mono Depth  & 29.63 & 0.838 & 0.471 & 6.984 & 0.142 & 28.71 & 0.834 & 0.475 & 7.649 & 0.153 \\
\bottomrule

\end{tabular}
} 
\label{tab:argosupp}
\end{table*}

\begin{table*}
\caption{Quantitative comparison of NeRF++ on each sequence of KITTI dataset. The best results are bolded.}
\centering
\resizebox{\textwidth}{!}{%
\begin{tabular}{lllccccccccccccccc}
\toprule
& & & \multicolumn{5}{c}{Dense} & \multicolumn{5}{c}{Sparse} \\ Method & Sequence& Depth Supervision & PSNR$\uparrow$ & SSIM$\uparrow$ & LPIPS$\downarrow$ & RMSE$\downarrow$ & Absrel$\downarrow$ & PSNR$\uparrow$ & SSIM$\uparrow$ & LPIPS$\downarrow$ & RMSE$\downarrow$ & Absrel$\downarrow$ \\
\cmidrule(lr){1-1}
\cmidrule(lr){2-2}
\cmidrule(lr){3-3}
\cmidrule(lr){4-8}
% \cmidrule(lr){8-12}
\cmidrule(lr){9-13}
\multirow{25}{*}{NeRF++~\cite{zhang2020nerf++}} & \multirow{5}{*}{(1)} & RGB-Only         & \textbf{20.64} & \textbf{0.657} & \textbf{0.512} & 51.983 & 4.214 & 17.88 & 0.598 & 0.534 & 53.995 & 4.372 \\
 &  & GT Depth         & 19.98 & 0.621 & 0.556 & \textbf{1.490}  & \textbf{0.061} & 19.39 & 0.622 & 0.543 & \textbf{1.529}  & \textbf{0.058} \\
 &  & Mono Depth       & 20.41 & 0.639 & 0.534 & 2.569  & 0.077 & 19.04 & 0.600 & \textbf{0.560} & 2.731  & 0.085 \\
 &  & Depth Completion & 20.03 & 0.623 & 0.550 & 1.581  & 0.066 & \textbf{19.37} & 0.616 & 0.544 & 1.594  & 0.066 \\
 &  & Stereo Depth     & 18.92 & 0.581 & 0.587 & 3.235  & 0.084 & 19.34 & \textbf{0.617} & 0.544 & 1.658  & 0.066 \\
\cmidrule{2-13}
 & \multirow{5}{*}{(2)}  & RGB-Only         & 19.83 & 0.234 & 0.539 & 42.549 & 2.938 & 16.50 & 0.503 & 0.553 & 57.436 & 4.998 \\
 &  & GT Depth         & 20.09 & 0.567 & 0.539 & \textbf{1.942}  & \textbf{0.047} & 18.84 & 0.540 & 0.549 & \textbf{1.208}  & \textbf{0.050} \\
 &  & Mono Depth       & \textbf{20.27} & 0.570 & 0.537 & 2.107  & 0.074 & 18.63 & 0.540 & 0.553 & 2.147  & 0.078 \\
 &  & Depth Completion & 20.19 & \textbf{0.571} & 0.534 & 1.282  & 0.051 & \textbf{18.90} & \textbf{0.543} & \textbf{0.548} & 1.370  & 0.057 \\
 &  & Stereo Depth     & 20.18 & \textbf{0.571} & \textbf{0.532} & 1.356  & 0.052 & 18.58 & 0.525 & 0.574 & 1.530  & 0.068 \\
 \cmidrule{2-13}
 & \multirow{5}{*}{(3)} & RGB-Only         & \textbf{19.83} & \textbf{0.517} & \textbf{0.566} & 42.549 & 2.938 & 16.91 & 0.452 & \textbf{0.588} & 55.046 & 4.735 \\
 &  & GT Depth         & 19.59 & 0.503 & 0.583 & \textbf{2.110}  & \textbf{0.087} & 17.99 & 0.472 & 0.594 & \textbf{2.292}  & \textbf{0.111} \\
 &  & Mono Depth       & 19.55 & 0.501 & 0.582 & 2.847  & 0.118 & 17.77 & \textbf{0.471} & 0.595 & 2.953  & 0.127 \\
 &  & Depth Completion & 19.64 & 0.506 & 0.580 & 2.296  & 0.100 & 18.03 & 0.476 & 0.592 & 2.398  & 0.110 \\
 &  & Stereo Depth     & 19.67 & 0.507 & 0.578 & 2.233  & 0.108 & \textbf{18.16} & 0.476 & 0.590 & 2.352  & 0.117 \\
 \cmidrule{2-13}
 & \multirow{5}{*}{(4)} & RGB-Only         & \textbf{20.26} & \textbf{0.585} & \textbf{0.559} & 46.588 & 3.704 & 17.78 & 0.544 & 0.577 & 53.181 & 4.544 \\
 &  & GT Depth         & 20.08 & 0.576 & 0.577 & \textbf{2.128}  & \textbf{0.096} & 18.66 & \textbf{0.554} & 0.585 & \textbf{2.300}  & \textbf{0.110} \\
 &  & Mono Depth       & 20.00 & 0.574 & 0.579 & 2.913  & 0.117 & 18.63 & 0.551 & 0.586 & 2.985  & 0.133 \\
 &  & Depth Completion & 20.05 & 0.574 & 0.577 & 2.406  & 0.108 & \textbf{18.70} & 0.553 & \textbf{0.587} & 2.503  & 0.116 \\
 &  & Stereo Depth     & 20.01 & 0.573 & 0.577 & 2.319  & 0.109 & 18.65 & \textbf{0.554} & 0.586 & 2.426  & 0.117 \\
 \cmidrule{2-13}
 & \multirow{5}{*}{(5)} & RGB-Only         & \textbf{20.91} & \textbf{0.608} & \textbf{0.549} & 59.522 & 5.792 & 18.94 & 0.578 & 0.558 & 61.611 & 6.148 \\
 &  & GT Depth         & 20.66 & 0.602 & 0.560 & \textbf{1.900}  & \textbf{0.098} & 19.60 & \textbf{0.583} & 0.572 & \textbf{2.083}  & \textbf{0.114} \\
 &  & Mono Depth       & 20.51 & 0.596 & 0.566 & 2.655  & 0.122 & \textbf{19.62} & 0.580 & 0.576 & 2.667  & 0.130 \\
 &  & Depth Completion & 20.60 & 0.601 & 0.562 & 2.104  & 0.111 & 19.51 & 0.580 & \textbf{0.577} & 2.245  & 0.122 \\
 &  & Stereo Depth     & 20.58 & 0.600 & 0.563 & 2.138  & 0.110 & 19.52 & 0.577 & 0.575 & 2.343  & 0.123 \\
\bottomrule
\end{tabular}
} 
\label{tab:nerfppkitti}
\end{table*}

\begin{figure*}
    \centering
    \includegraphics[width=0.95\textwidth]{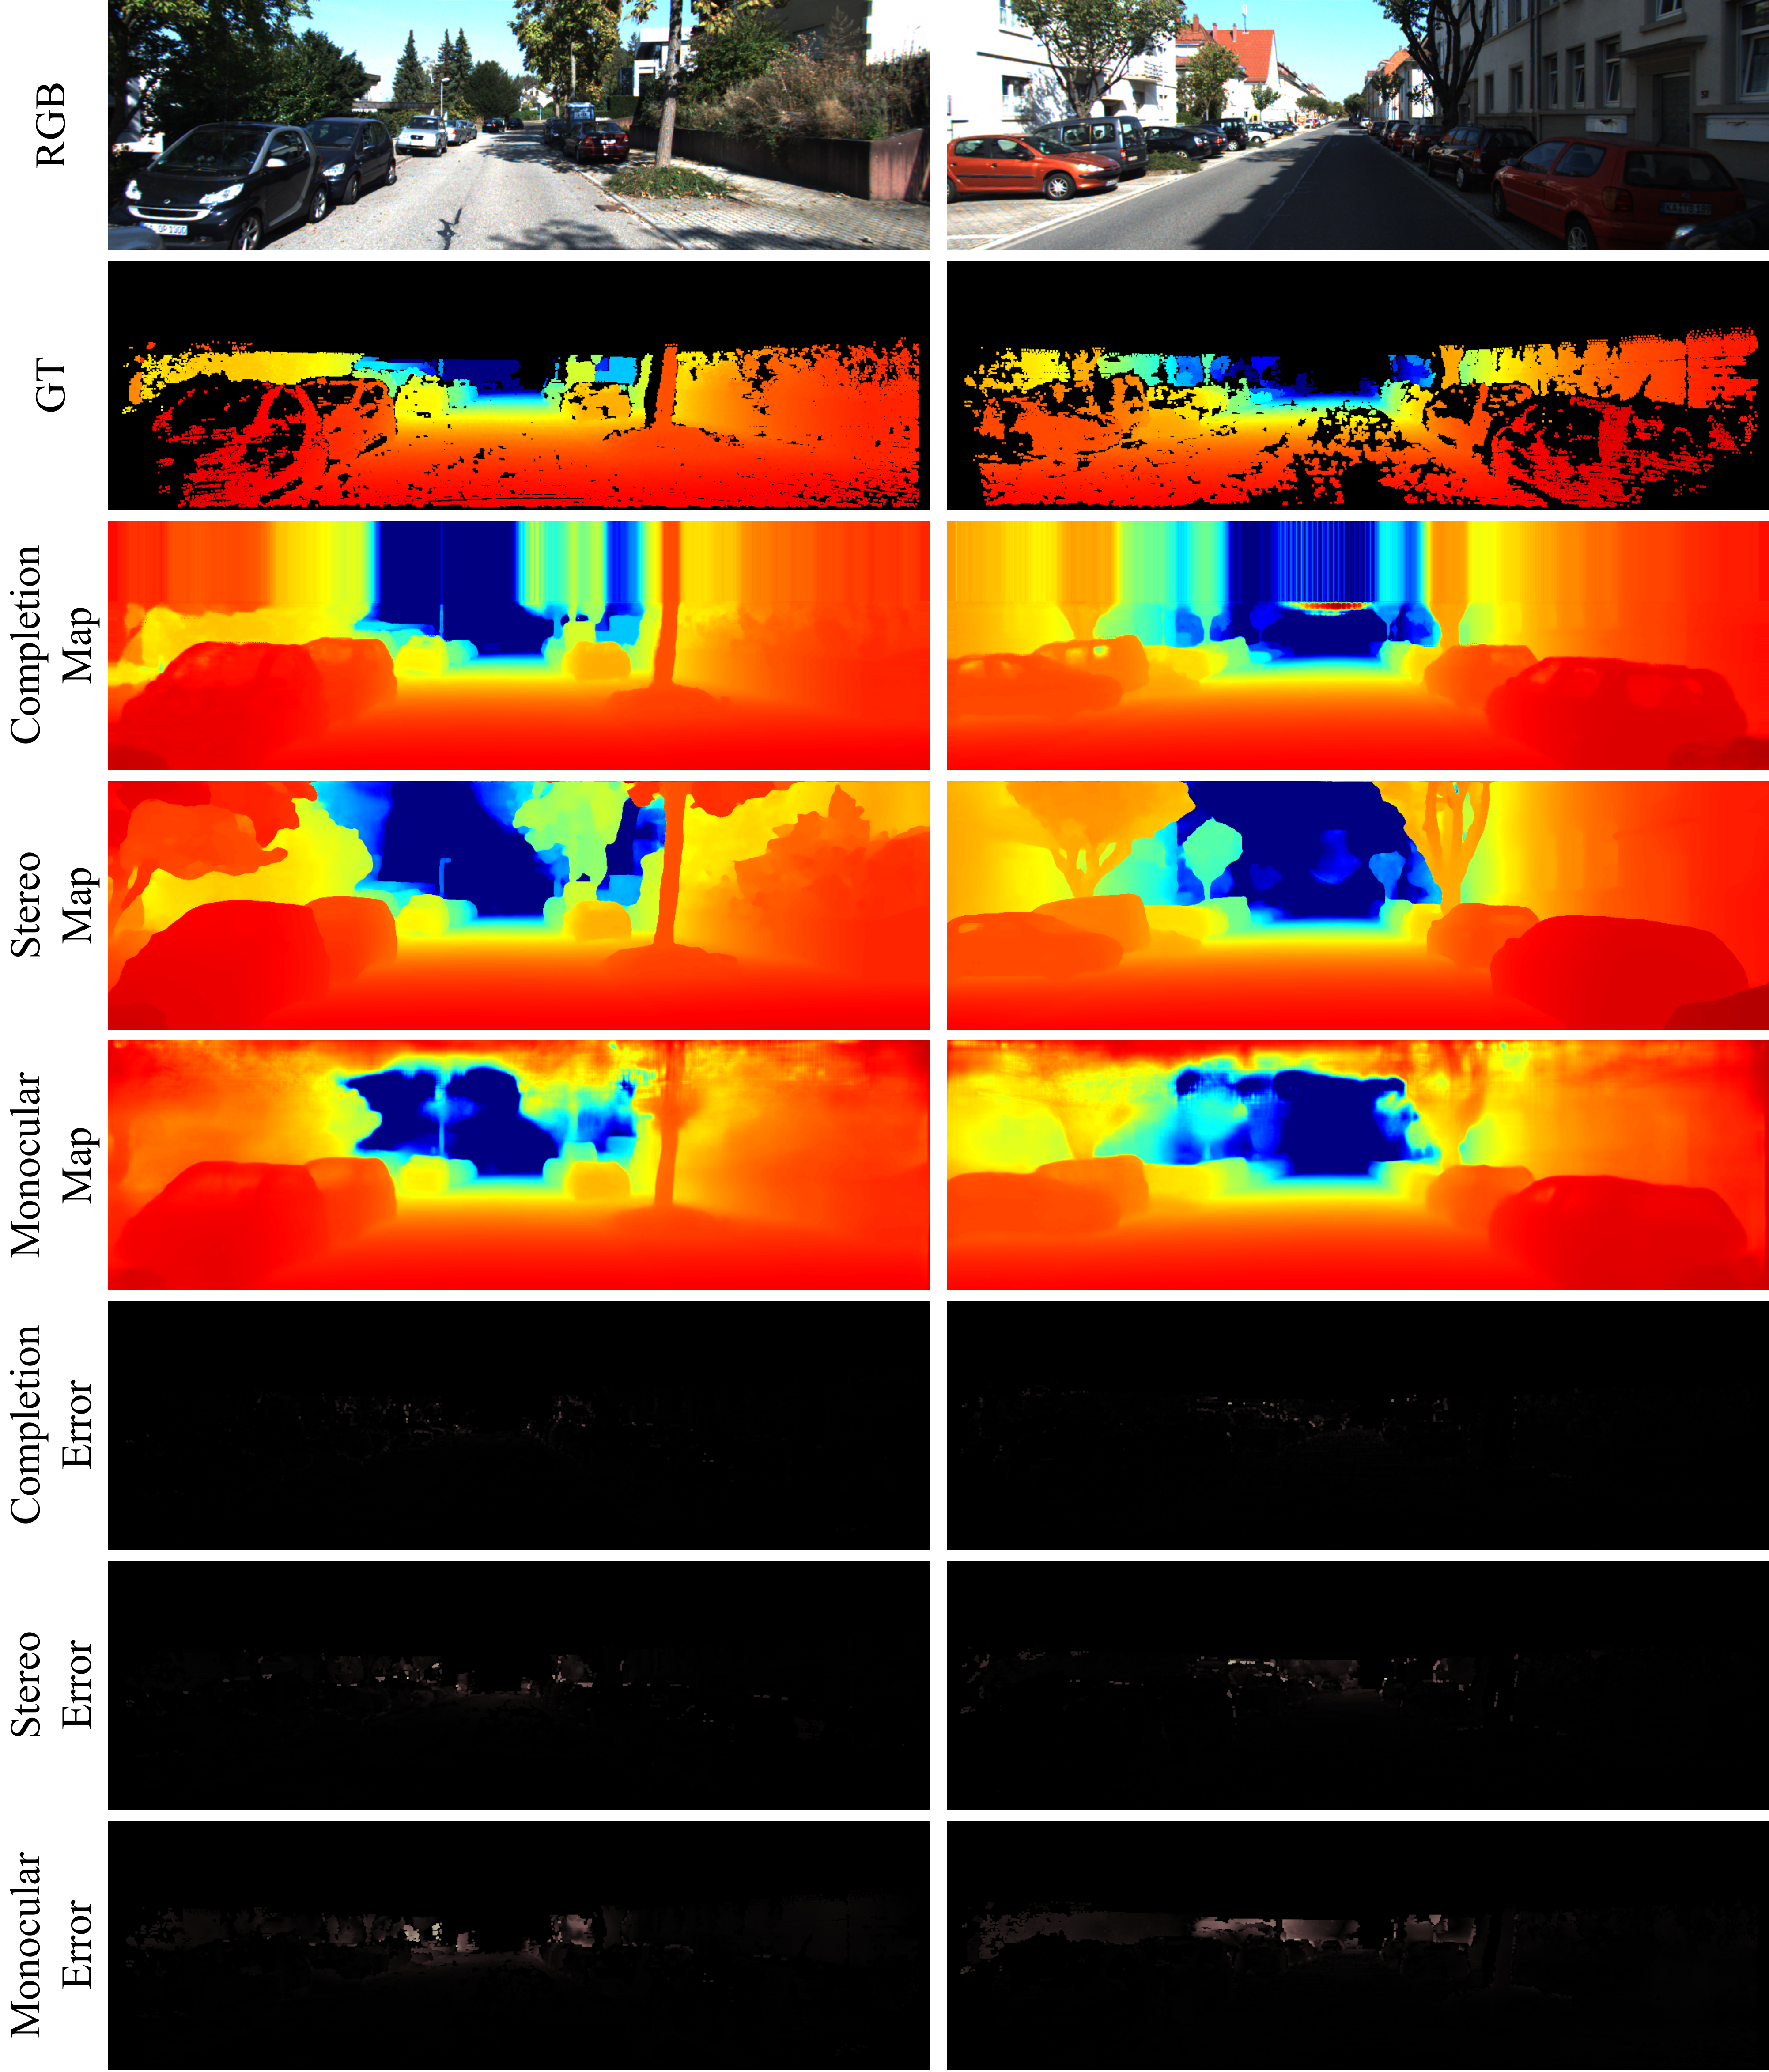}
    \caption{Qualitative results on the KITTI dataset with different depth recovery methods. White and blue denotes larger error and further distance in the error map and colorized depth map, respectively. For depth recovery accuracy, depth completion has the best accuracy in gt valid area then goes with binocular depth estimation and monocular depth estimation}
    \label{fig:KITTI_res}
    % \vspace{-0.1in}
\end{figure*}
